# Supplementary material for: Deep Equilibrium Object Detection
Source: arXiv:2308.09564 source file (2023-08-18)
Supplement: Supplementary file 1 [file appendix.tex]

\documentclass[10pt,twocolumn,letterpaper]{article}

\usepackage{iccv}
\usepackage{times}
\usepackage{epsfig}
\usepackage{graphicx}
\usepackage{amsmath}
\usepackage{amssymb}
\usepackage{booktabs}
\usepackage{times}
\usepackage{mathtools}
\usepackage{amsthm}
\usepackage{microtype}
\usepackage{subfig}
\usepackage{enumitem}
\usepackage{mmstyle}
\usepackage{algorithm}
\usepackage{bm}
\usepackage{algorithmic}
\usepackage{float}
\usepackage{listings}
\usepackage{makecell}  % \Xhline
\usepackage{diagbox} % diagonal table cell
\usepackage{multirow}
\usepackage{bbm}
% Include other packages here, before hyperref.

% If you comment hyperref and then uncomment it, you should delete
% egpaper.aux before re-running latex.  (Or just hit 'q' on the first latex
% run, let it finish, and you should be clear).
\usepackage[pagebackref=true,breaklinks=true,letterpaper=true,colorlinks,bookmarks=false]{hyperref}

\usepackage[table]{xcolor}
\definecolor{detcolor}{gray}{.9}

% \definecolor{bestcolor}{RGB}{238, 255, 238}
\definecolor{bestcolor}{gray}{.9}

% %%%%%%%%%%%%%% ConvNext %%%%%%%%

\newlength\savewidth
  
% %%%%%%%%%%%%%%%%%%% MAE %%%%%%%%%%
\newcolumntype{x}[1]{>{\centering\arraybackslash}p{#1pt}}
\newcolumntype{y}[1]{>{\raggedright\arraybackslash}p{#1pt}}
\newcolumntype{z}[1]{>{\raggedleft\arraybackslash}p{#1pt}}
\renewcommand{\paragraph}[1]{\vspace{1.25mm}\noindent\textbf{#1}}
\definecolor{deemph}{gray}{0.6}

\usepackage[capitalize]{cleveref}
\crefname{section}{Sec.}{Secs.}
\Crefname{section}{Section}{Sections}
\crefname{table}{Tab.}{Tabs.}
\Crefname{table}{Table}{Tables}

 % *** Enter the ICCV Paper ID here

% Pages are numbered in submission mode, and unnumbered in camera-ready
\ificcvfinal\pagestyle{empty}\fi

\begin{document}

%%%%%%%%% TITLE
\title{DEQDet: Object Detection with Deep Equilibrium Decoders}

\author{First Author\\
Institution1\\
Institution1 address\\
{\tt\small firstauthor@i1.org}
% For a paper whose authors are all at the same institution,
% omit the following lines up until the closing ``}''.
% Additional authors and addresses can be added with ``\and'',
% just like the second author.
% To save space, use either the email address or home page, not both
\and
Second Author\\
Institution2\\
First line of institution2 address\\
{\tt\small secondauthor@i2.org}
}

\maketitle
% Remove page # from the first page of camera-ready.
\ificcvfinal\thispagestyle{empty}\fi

\newpage
\appendix

%%%%%%%%% TITLE
\title{DEQDet: Object Detection with Deep Equilibrium Decoders}

\author{First Author\\
Institution1\\
Institution1 address\\
{\tt\small firstauthor@i1.org}
% For a paper whose authors are all at the same institution,
% omit the following lines up until the closing ``}''.
% Additional authors and addresses can be added with ``\and'',
% just like the second author.
% To save space, use either the email address or home page, not both
\and
Second Author\\
Institution2\\
First line of institution2 address\\
{\tt\small secondauthor@i2.org}
}

\maketitle
% Remove page # from the first page of camera-ready.
\ificcvfinal\thispagestyle{empty}\fi

\newpage
\appendix

{\small
\bibliographystyle{ieee_fullname}
\bibliography{main}
}

{\small
\bibliographystyle{ieee_fullname}
\bibliography{main}
}
\end{document}
